# Supplementary material for: A Survey and Benchmark of Automatic Surface Reconstruction from Point Clouds
Source: arXiv:2301.13656 source file (2024-12-02)
Supplement: Supplementary file 1 [file suppmat.tex]

\documentclass[10pt,journal,compsoc]{ieee/IEEEtran}

%
% If IEEEtran.cls has not been installed into the LaTeX system files,
% manually specify the path to it like:
% \documentclass[10pt,journal,compsoc]{../sty/IEEEtran}

% Some very useful LaTeX packages include:
% (uncomment the ones you want to load)

% *** MISC UTILITY PACKAGES ***
%
%\usepackage{ifpdf}
% Heiko Oberdiek's ifpdf.sty is very useful if you need conditional
% compilation based on whether the output is pdf or dvi.
% usage:
% \ifpdf
%   % pdf code
% \else
%   % dvi code
% \fi
% The latest version of ifpdf.sty can be obtained from:
% http://www.ctan.org/pkg/ifpdf
% Also, note that IEEEtran.cls V1.7 and later provides a builtin
% \ifCLASSINFOpdf conditional that works the same way.
% When switching from latex to pdflatex and vice-versa, the compiler may
% have to be run twice to clear warning/error messages.

% *** CITATION PACKAGES ***
%
\ifCLASSOPTIONcompsoc
  % IEEE Computer Society needs nocompress option
  % requires cite.sty v4.0 or later (November 2003)
  \usepackage[nocompress]{cite}
\else
  % normal IEEE
  \usepackage{cite}
\fi
% cite.sty was written by Donald Arseneau
% V1.6 and later of IEEEtran pre-defines the format of the cite.sty package
% \cite{} output to follow that of the IEEE. Loading the cite package will
% result in citation numbers being automatically sorted and properly
% "compressed/ranged". e.g., [1], [9], [2], [7], [5], [6] without using
% cite.sty will become [1], [2], [5]--[7], [9] using cite.sty. cite.sty's
% \cite will automatically add leading space, if needed. Use cite.sty's
% noadjust option (cite.sty V3.8 and later) if you want to turn this off
% such as if a citation ever needs to be enclosed in parenthesis.
% cite.sty is already installed on most LaTeX systems. Be sure and use
% version 5.0 (2009-03-20) and later if using hyperref.sty.
% The latest version can be obtained at:
% http://www.ctan.org/pkg/cite
% The documentation is contained in the cite.sty file itself.
%
% Note that some packages require special options to format as the Computer
% Society requires. In particular, Computer Society  papers do not use
% compressed citation ranges as is done in typical IEEE papers
% (e.g., [1]-[4]). Instead, they list every citation separately in order
% (e.g., [1], [2], [3], [4]). To get the latter we need to load the cite
% package with the nocompress option which is supported by cite.sty v4.0
% and later. Note also the use of a CLASSOPTION conditional provided by
% IEEEtran.cls V1.7 and later.

% *** GRAPHICS RELATED PACKAGES ***
%
\ifCLASSINFOpdf
  % \usepackage[pdftex]{graphicx}
  % declare the path(s) where your graphic files are
  % \graphicspath{{../pdf/}{../jpeg/}}
  % and their extensions so you won't have to specify these with
  % every instance of \includegraphics
  % \DeclareGraphicsExtensions{.pdf,.jpeg,.png}
\else
  % or other class option (dvipsone, dvipdf, if not using dvips). graphicx
  % will default to the driver specified in the system graphics.cfg if no
  % driver is specified.
  % \usepackage[dvips]{graphicx}
  % declare the path(s) where your graphic files are
  % \graphicspath{{../eps/}}
  % and their extensions so you won't have to specify these with
  % every instance of \includegraphics
  % \DeclareGraphicsExtensions{.eps}
\fi
\hyphenation{op-tical net-works semi-conduc-tor}

\input{settings/packages}
\input{settings/newcommands}

\usepackage{alphalph}

\begin{document}
\include{acronyms}

%
% paper title
% Titles are generally capitalized except for words such as a, an, and, as,
% at, but, by, for, in, nor, of, on, or, the, to and up, which are usually
% not capitalized unless they are the first or last word of the title.
% Linebreaks \\ can be used within to get better formatting as desired.
% Do not put math or special symbols in the title.
\title{Supplementary Material: A Survey and Benchmark of Automatic Surface Reconstruction from Point Clouds}

\author{Raphael~Sulzer,
        Renaud~Marlet,
        Bruno~Vallet~and~Loic~Landrieu}

% The paper headers
% \markboth{Journal of \LaTeX\ Class Files,~Vol.~14, No.~8, August~2015}%
% {Shell \MakeLowercase{\textit{et al.}}: Bare Demo of IEEEtran.cls for Computer Society Journals}

% make the title area
\maketitle

% To allow for easy dual compilation without having to reenter the
% abstract/keywords data, the \IEEEtitleabstractindextext text will
% not be used in maketitle, but will appear (i.e., to be "transported")
% here as \IEEEdisplaynontitleabstractindextext when the compsoc 
% or transmag modes are not selected <OR> if conference mode is selected 
% - because all conference papers position the abstract like regular
% papers do.
\IEEEdisplaynontitleabstractindextext
% \IEEEdisplaynontitleabstractindextext has no effect when using
% compsoc or transmag under a non-conference mode.

% For peer review papers, you can put extra information on the cover
% page as needed:
% \ifCLASSOPTIONpeerreview
% \begin{center} \bfseries EDICS Category: 3-BBND \end{center}
% \fi
%
% For peerreview papers, this IEEEtran command inserts a page break and
% creates the second title. It will be ignored for other modes.
\IEEEpeerreviewmaketitle

% In this supplementary document, we first provide implementation details (\secref{sec:imp_details}), additional information about the datasets that we use (\secref{sec:datasets}), 
{In this supplementary document, we provide additional information about the datasets we used in our benchmark and additional results. All the datasets and the evaluation code for our benchmark are available on GitHub: \url{https://github.com/raphaelsulzer/dsr-benchmark}}

\section{Datasets}
\subsection{Berger \etal}
% Please add the following required packages to your document preamble:
% \usepackage{booktabs}
% \usepackage{graphicx}
\begin{table*}
\centering
\caption[Scanning configurations for Berger \etal benchmark]{\textbf{Scanning configurations for Berger \etal benchmark:} We show the five different scanner configurations used in our modified version of the Berger et al.'s scanning procedure. We use the resulting scans to evaluate object-level reconstruction with varying point-cloud defects and for training data generation. For the low resolution (LR) scans the scanning process results in $1000$ to $3000$ points per shape, and for the high resolution (HR), the scanning process yields around $10\,000$ to $30\,000$ points.}
\resizebox{0.9\textwidth}{!}{%
\begin{tabular}{@{}lccccc@{}}
\toprule
\multicolumn{1}{l}{} & \textbf{Low res. (LR)} & \textbf{High res. (HR)} & \textbf{HR + noise (HRN)} & \textbf{HR + outliers (HRO)} & \textbf{HR + noise + outliers (HRNO)} \\ \midrule
Camera resolution x, y & 50, 50 & 100, 100 & 100, 100 & 100, 100 & 100, 100 \\
Scanner positions & 5 & 10 & 10 & 10 & 10 \\
Min/max range & 70/300 & 70/300 & 70/300 & 70/300 & 70/300 \\
Additive noise & 0 & 0 & 0.5 & 0 & 0.5 \\
Outliers (\%) & 0 & 0 & 0 & 0.1 & 0.1 \\ \bottomrule
\end{tabular}%
}
\label{tab:berger_confs}
\end{table*}
We use the range scanning procedure from the surface reconstruction benchmark of Berger \etal \cite{Berger_benchmark}. To this end, we modified 
%\footnote{Our modified version of the benchmark code will be available on Github.\\~\\} 
their provided code to export the camera positions of the scanning process along with the point cloud. Our modified version of the code is available on Github: \url{https://github.com/raphaelsulzer/reconbench-CMake}. We choose five different scanner settings, detailed in \tabref{tab:berger_confs} and visible in the first row of \figref{fig:ch2:optim_results} to scan each test shape shown in \figref{fig:gt:berger}.

\subsection{ModelNet10 and ShapeNet}
\input{figures/gt/gt_figure}
We show example shapes for all classes of ShapeNet in \figref{fig:gt:shapenet} and example shapes for ModelNet for the $6$ out of $10$ classes which are not represented in ShapeNet in \figref{fig:gt:modelnet}.

\section{Benchmark setup}
\begin{table*}
\caption[Benchmark setup]{
	\textbf{Benchmark setup:} 
We show an overview of our experimental setup. In E1 to E4, we train surface reconstruction methods on noisy point clouds of ShapeNet.  In E1, we test on the ShapeNet test set. In E2, we test on ShapeNet, but from denser point clouds with noise and outliers. In E3, we test on the simpler ModelNet objects with the same sampling as in E1. In E4, we train the methods on the simpler ModelNet dataset and test on ShapeNet, both with the same sampling as in E1. In E5, we test optimization-based methods on synthetic range scans of the Berger \etal dataset. And finally, in E6, we compare learning- and optimization-based methods on the same dataset (synthetic MVS scans of the Berger \etal dataset).
}
\begin{adjustbox}{max width=\textwidth}
\footnotesize
\centering
\begin{tabular}{ccccccccccccc}
\toprule
            & \multicolumn{6}{c}{\textbf{\textit{Training set}}}        &  \multicolumn{6}{c}{\textbf{\textit{Test set}}}                                         \\
\textbf{Experiment}  & \textbf{Name}          & \textbf{\#~shapes} & \textbf{complexity}    & \textbf{\#~points} &       \textbf{$\sigma$~noise} & \textbf{\%~outliers}    & \textbf{Name}    & \textbf{\#~shapes} & \textbf{complexity}    & \textbf{\#~points} & \textbf{$\sigma$~noise} & \textbf{\%~outliers}   \\ \midrule
1           & ShapeNet      & $30,661$  & $\star\star$  & $3,000$           & $0.005$       & $0$               & ShapeNet      & $1,300$   & $\star\star$  & $3,000$   & $0.005$       & $0$           \\
2           & ShapeNet      & $30,661$  & $\star\star$  & $3,000$           & $0.005$       & $0$               & ShapeNet      & $1,300$   & $\star\star$  & $10k$  & $0.005$       & $10$          \\
3           & ShapeNet      & $30,661$  & $\star\star$  & $3,000$           & $0.005$       & $0$               & ModelNet      & $506$     & $\star$       & $3,000$   & $0.005$       & $0$           \\
% 4           & ShapeNet      & $30,661$  & $\star\star$  & $3,000$           & $0.005$       & $0$               & Berger~\etal  & $5$       & $\star\star$  & $3,000$   & $0.005$       & $0$           \\
4           & ModelNet      & $3,979$   & $\star$       & $3,000$           & $0.005$       & $0$               & ShapeNet      & $1,300$   & $\star\star$  & $3,000$   & $0.005$       & $0$           \\ 
% 6           & SRD           & $3,979$   & $\star\star\star$& $500-50k$      & $0.000-0.025$ & $0-50$            & ETH3D         & $1,300$   & $\star\star$  & $3,000$   & $0.005$       & $0$           \\
\midrule
5           & \multicolumn{6}{c}{--}                                                           & Berger~\etal  & $5$       & $\star\star$  &\multicolumn{3}{c}{see \tabref{tab:berger_confs}} \\
\midrule
6           &  ShapeNet      & $30,661$  & $\star\star$  & $3,000$           & $0.005$       & $0$   & Berger~\etal  & $5$       & $\star\star$  & $3,000$   & $0.005$       & $0$                   \\
\midrule
7           &  ShapeNet      & $30,661$  & $\star\star$  & $3,000$           & $0.005$       & $0$   & Real  & $3$       & $\star\star\star$  & $10,000$   & \emph{variable}       & \emph{variable}                   \\
\bottomrule
% 5           & FamousThingi  & $50$      & $\star\star$  & $300$-$30,000$    & $0.005$       & $0$               & Berger~\etal  & $1,300$   & $10,000$  & $0.005$       & $10$          \\ \bottomrule
% 6           & FamousThingi  & $50$      & $\star\star$  & $300$-$30,000$    & $0.005$       & $0$               & ETH3D         & $3$       & $10,000$  & $0.005$       & $10$          \\ \bottomrule
\end{tabular}
\end{adjustbox}
\label{ch2:tab:benchmark_supp}
\end{table*}

We show a detailed overview of our benchmark setup on \tabref{ch2:tab:benchmark_supp}.

\section{Additional results}
\input{figures/optim_results/optim_results} 
\begin{figure*}
% \captionsetup{justification=centering,font=tiny} % this is for the figure captions
\captionsetup[sub]{labelfont=scriptsize,textfont=scriptsize,justification=centering}
    \centering
    \newcommand{\mywidth}{0.13\textwidth}
    \definetrim{mytrim}{50 50 50 50}
    \begin{tabular}{@{}c@{}c@{}c@{}c@{}c@{}c@{}c|@{}c@{}}
        %  &
        %  &
        %  & \subfloat[Input]{    \includegraphics[width=\mywidth]{figures/learning_optim/input.jpg}\label{fig:lo:in}}
        %  & \subfloat[GT]{    \includegraphics[width=\mywidth]{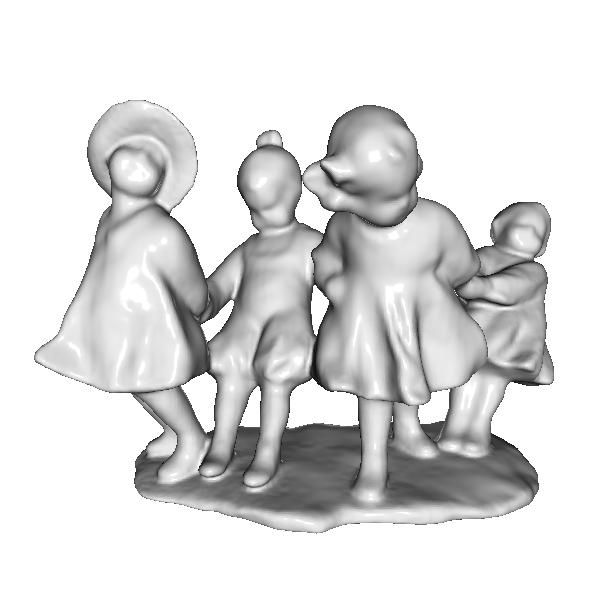}\label{fig:lo:gt}}
        %  &
        %  &
        %  \\
         \rotatebox{90}{\hspace{0mm}Learning}
         &
         &  \subfloat[CONet2D]{    \includegraphics[width=\mywidth,mytrim]{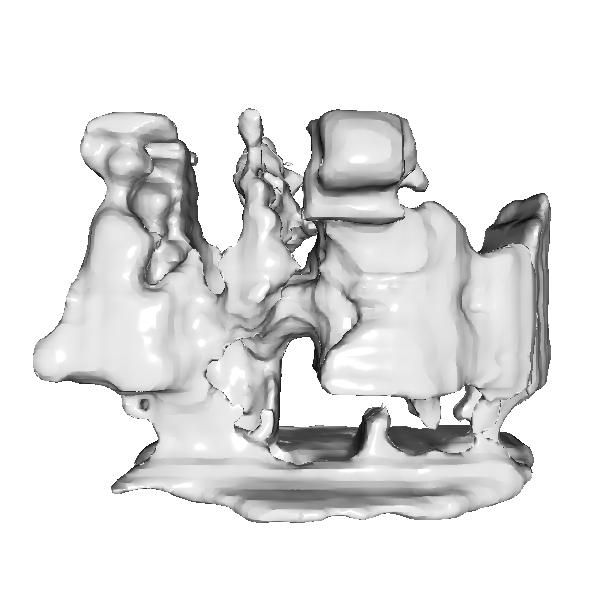}\label{fig:lo:onet2}}
         &  \subfloat[CONet3D]{    \includegraphics[width=\mywidth,mytrim]{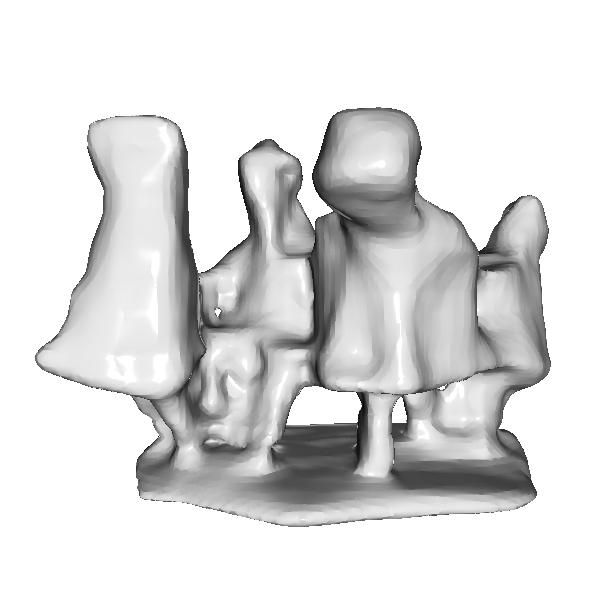}\label{fig:lo:onet3}}
         &  \subfloat[SAP]{    \includegraphics[width=\mywidth,mytrim]{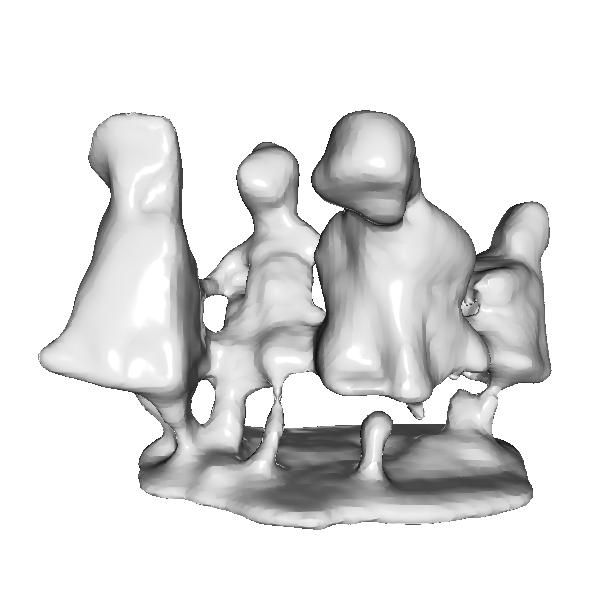}\label{fig:lo:sap}}
         &  \subfloat[DGNN]{    \includegraphics[width=\mywidth,mytrim]{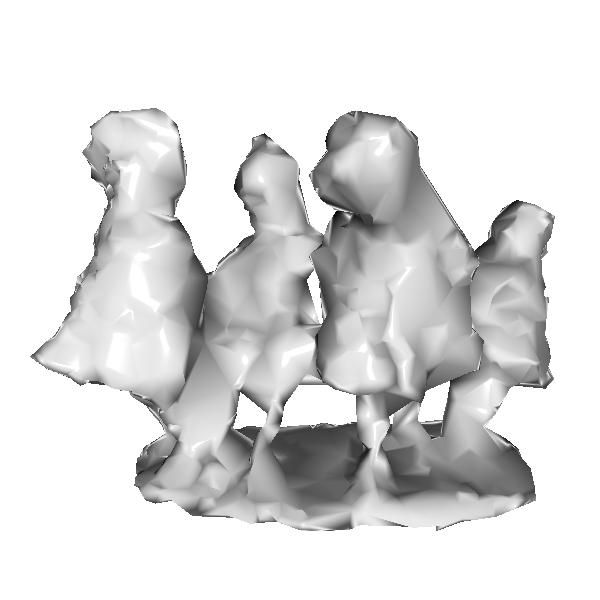}\label{fig:lo:dgnn}}         
         &  \subfloat[POCO]{    \includegraphics[width=\mywidth,mytrim]{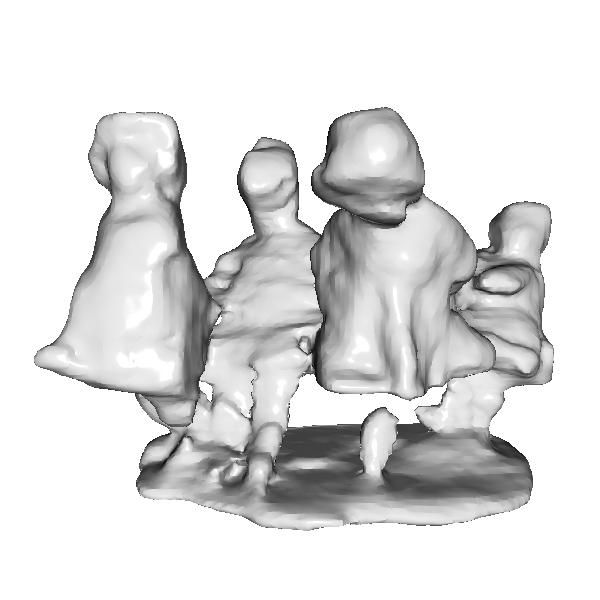}\label{fig:lo:poco}}
         & \subfloat[Input]{    \includegraphics[width=\mywidth,mytrim]{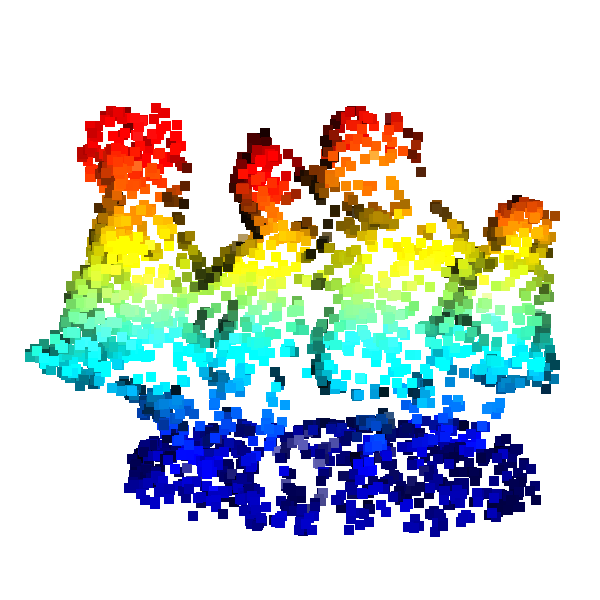}\label{fig:lo:in}}
         \\
         \rotatebox{90}{\hspace{-1mm}Optimization}
         & \subfloat[IGR]{    \includegraphics[width=\mywidth,mytrim]{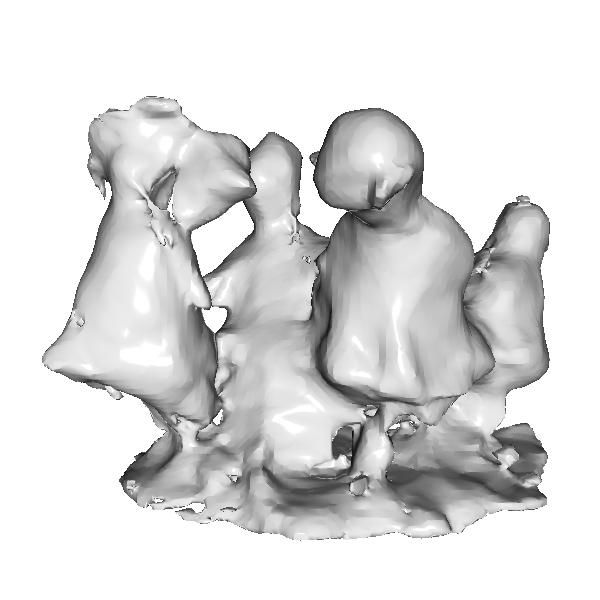}\label{fig:lo:igr}}
         &  \subfloat[LIG]{    \includegraphics[width=\mywidth,mytrim]{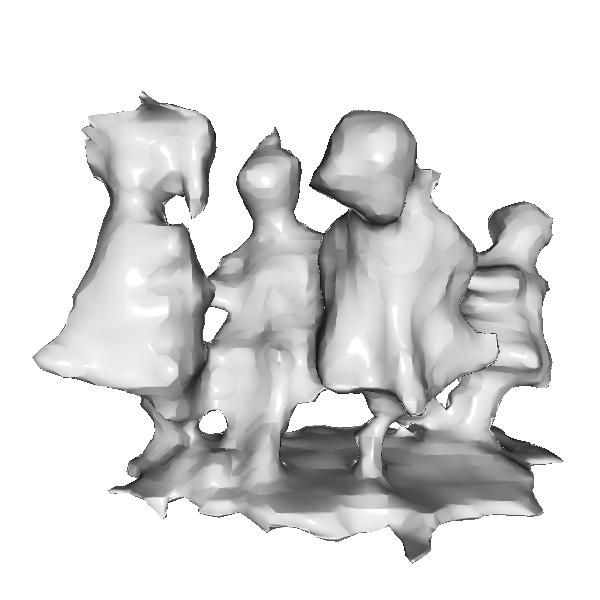}\label{fig:lo:lig}}
         &  \subfloat[P2M]{    \includegraphics[width=\mywidth,mytrim]{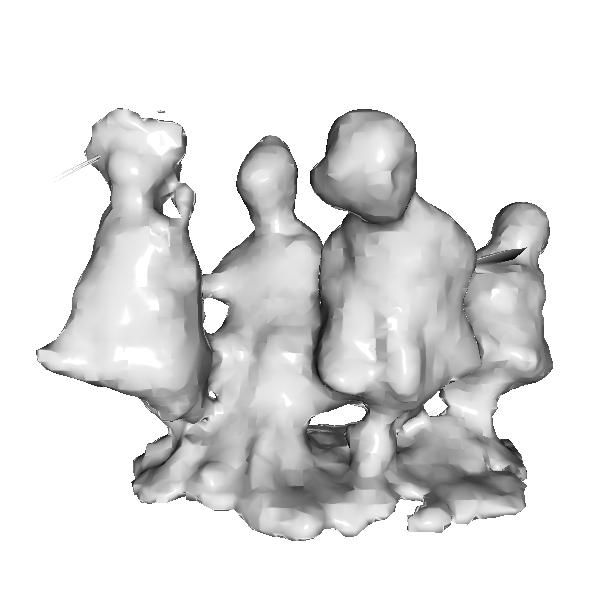}\label{fig:lo:p2m}}
         &  \subfloat[SAP\optim]{    \includegraphics[width=\mywidth,mytrim]{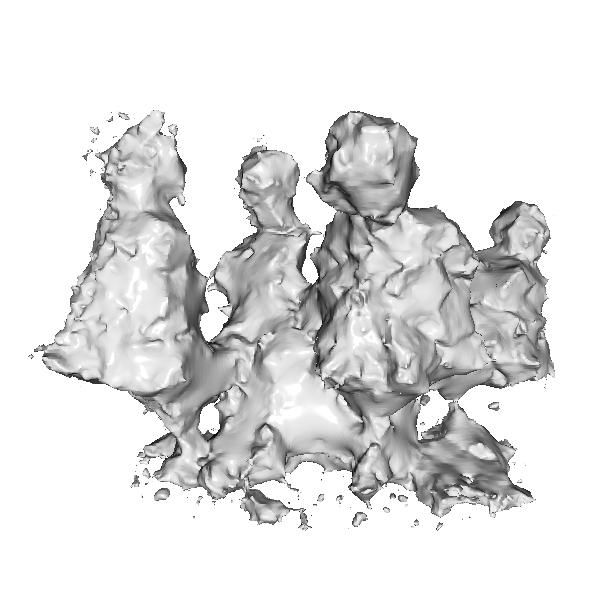}\label{fig:lo:sap2}}
         &  \subfloat[SPSR]{    \includegraphics[width=\mywidth,mytrim]{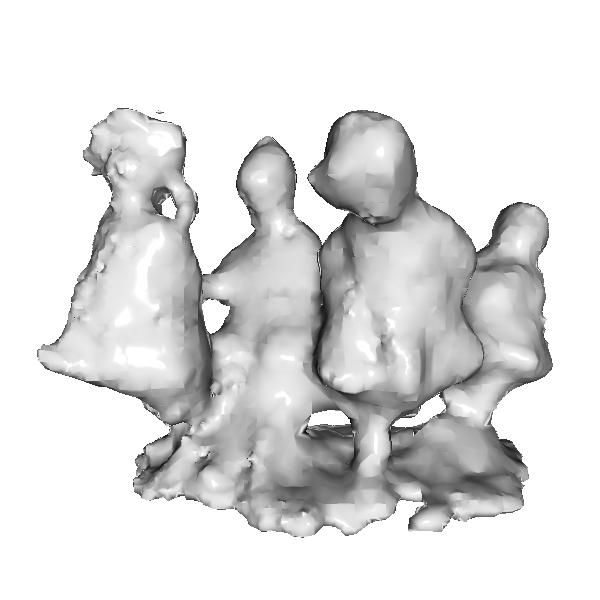}\label{fig:lo:spsr}}         
         &  \subfloat[RESR]{    \includegraphics[width=\mywidth,mytrim]{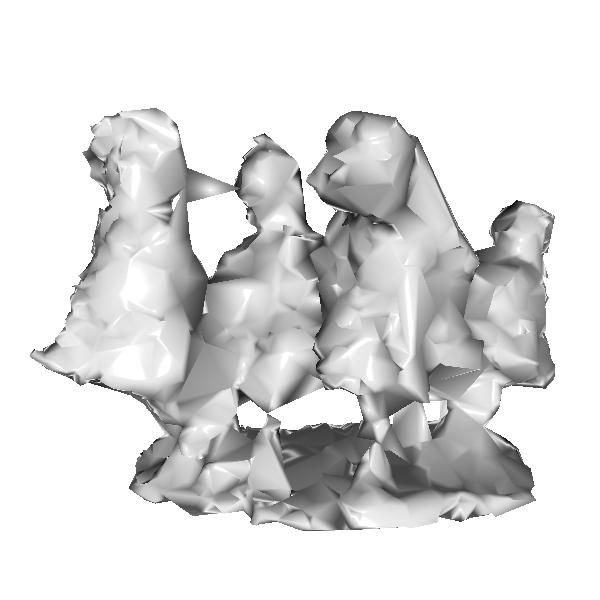}\label{fig:lo:lab}}   
         & \subfloat[GT]{    \includegraphics[width=\mywidth,mytrim]{figures/learning_optim/gt.jpg}\label{fig:lo:gt}}
    \end{tabular}
\caption[Learning- vs. optimization-based reconstructions]{\textbf{Learning- vs. optimization-based reconstructions (E6):} We show reconstructions of \emph{dancing children} from Berger \etal from a low resolution input point cloud with noise (\subref{fig:lo:in}) and the ground truth shape (\subref{fig:lo:gt}). The methods used in the first row (\subref{fig:lo:onet2} - \subref{fig:lo:poco})  were trained on ShapeNet, on point clouds with the same sampling as the one used here. In the second row (\subref{fig:lo:igr} - \subref{fig:lo:spsr}) we show the reconstructions for the same shape (from the same sampling) from optimization-based methods.
}
    \label{fig:ch2:learning_optim}
\end{figure*} 
We show qualitative results of Experiment 6 and 7 in \figref{fig:ch2:optim_results} and \figref{fig:ch2:learning_optim}, respectively.

\balance

\bibliographystyle{ieee/IEEEtran} 
\bibliography{ieee/IEEEabrv,references}

\end{document}
